# Supplementary material for: Virtual Elastic Tether: a New Approach for Multi-agent Navigation in Confined Aquatic Environments
Source: arXiv:2403.10629 source file (2024-08-14)
Supplement: Supplementary file 1 [file Appendix.tex]

% {\appendix[Proof of the Zonklar Equations]
% Use $\backslash${\tt{appendix}} if you have a single appendix:
% Do not use $\backslash${\tt{section}} anymore after $\backslash${\tt{appendix}}, only $\backslash${\tt{section*}}.
% If you have multiple appendixes use $\backslash${\tt{appendices}} then use $\backslash${\tt{section}} to start each appendix.
% You must declare a $\backslash${\tt{section}} before using any $\backslash${\tt{subsection}} or using $\backslash${\tt{label}} ($\backslash${\tt{appendices}} by itself
%  starts a section numbered zero.)}
\appendices
\section{Kinematic model}
The kinematic model of BlueROV2:
\begin{equation*}
    \begin{array}{cc}
\prescript{\mathcal{W}}{}{\bm{\dot x}}^U = \left[\begin{array}{cc}
            \prescript{\mathcal{B}}{\mathcal{W}}{{\bm{R}^U(\bm{\Theta})}}  & 0_{3 \times 3} \\
            0_{3 \times 3} & \prescript{\mathcal{B}}{\mathcal{W}}{{\bm{T}^U(\bm{\Theta})}}
                                        \end{array}\right] \left[ \begin{array}{c}
                                           \bm{\nu}^U_{x,y,z}\\
                                           \bm{\nu}^U_{\phi,\theta,\psi}
                            \end{array} \right] 
\end{array}
\end{equation*}
where $\bm{\nu}^U_{x,y,z} = [\nu^U_x,\nu^U_y,\nu^U_z]\top$, $\bm{\nu}^U_{\phi,\theta,\psi} = [\nu^U_{\phi},\nu^U_{\theta},\nu^U_{\psi}]\top$, and the transformation matrix $\prescript{\mathcal{B}}{\mathcal{W}}{{\bm{R}^U(\bm{\Theta})}}$ is given by 
\begin{equation*}
    \begin{array}{cc}
\prescript{\mathcal{B}}{\mathcal{W}}{{\bm{R}^U(\bm{\Theta})}} =\left[\begin{array}{ccc}
c \psi c \theta & -s \psi c \phi + c\psi s \theta s \phi & c \psi s \theta c \phi+s \psi s \phi \\
s \psi c \theta & c \psi c \phi + s \psi s \theta s \phi & -c \psi s \phi + s \psi s \theta c \phi \\
-s \theta & c \theta s \phi & c \theta c \phi
\end{array}\right]
    \end{array}
\end{equation*}
where $c$· stands for $cos($·$  )$ and $s$· stands for $sin($·$  )$. Similarly, the transformation matrix $\prescript{\mathcal{B}}{\mathcal{W}}{{\bm{T}^U(\bm{\Theta})}}$ is given by 

\begin{equation*}
    \begin{array}{cc}
\prescript{\mathcal{B}}{\mathcal{W}}{{\bm{T}^U(\bm{\Theta})}} = \left[ \begin{array}{ccc}
                              1 &  c\phi t\theta & c\phi t\theta  \\
                           0     &   c\phi  & -s\phi\\
                           0             & s\phi/c\theta        & c\phi /c\theta   
                            \end{array} \right]
    \end{array}
\end{equation*}
where $t$· stands for $tan($·$  )$.

The kinematic model of MallARD: 
\begin{equation*}
\begin{array}{cc}

    \prescript{\mathcal{W}}{}{\bm{\dot x}}^S =  \left[ \begin{array}{ccc}
                              -c\psi &   s\psi &   0\\
                           -s\psi      &   c\psi  & 0\\
                           0             & 0        &    1
                            \end{array} \right]  \left[\begin{array}{c}
                               \prescript{\mathcal{}}{}{{\nu}}^S_x   \\
                                  \prescript{\mathcal{}}{}{{\nu}}^S_y \\
                                  \prescript{\mathcal{}}{}{{\nu}}^S_\psi
                            \end{array}\right]
\end{array}
\end{equation*}

The terminology of \textbf{elasticity} in this context is somewhat metaphorical, a stretch of the conventional meaning (pun intended). In the realm of physical materials, elasticity refers to the property of a material to return to its original shape after being deformed. Here, however, we use it to describe the bounded yet adaptable behavior of the relative tether states between the robots. This conceptual 'elasticity' can be thought of in terms of the dynamic system represented by the following equation:
\begin{equation}
\begin{aligned}
    & \dot {\overline{\xi}} + \eta \cdot \overline{\xi} \leq 0, \quad \text{where} \quad \overline{\xi} = \xi - \xi_{\text{max}} \\
    \Rightarrow \quad &  \dot \xi + \eta \cdot \overline{\xi} \leq 0
\end{aligned}
\end{equation}

Here, $\overline{\xi}$ represents the deviation of the tether state from its maximum value. The condition $\dot {\overline{\xi}} + \eta \cdot \overline{\xi} \leq 0$ suggests a damping or stabilizing behavior, analogous to how an elastic material responds when stretched and released. In our system, this 'elastic' behavior is not about physical stretching but rather about maintaining the relative positions and movements of the robots within certain limits, reflecting a balance between flexibility and controlled constraint. This dynamic behavior, represented mathematically, encapsulates the essence of our metaphorical use of 'elasticity'.

% \begin{subequations}\label{eq:sys_kinematic}
% \begin{align}
%    U:  & \prescript{\mathcal{W}}{}{\bm{\dot x}}^U = \bm{J^U} \bm{\nu}^U \label{eq:sys_kinematic1}\\[5pt]
%    S:  & \prescript{\mathcal{W}}{}{\bm{\dot x}}^S = \bm{J^S} \bm{\nu}^S,\label{eq:sys_kinematic2}
% \end{align}
% \end{subequations}

% \begin{equation}\label{eq:E_e}
% \begin{array}{rrl}
%    U: &  \bm{e}^U_E|_{3:5} &=  \left[ \begin{array}{c}
%                               x^U_{d|z} - z^U_{k|z}\\
%                            x^U_{d|\phi} - z^U_{k|\phi}\\
%                            x^U_{d|\theta}- z^U_{k|\theta}
%                             \end{array} \right]  \\[16pt]
%    S: &   \bm{e}^S_E &=  \left[ \begin{array}{c}
%                               x^S_{d|x} - z^S_{k|x}\\
%                            x^S_{d|y} - z^S_{k|y}\\
%                            x^S_{d|\psi}- z^S_{k|\psi}
%                             \end{array} \right] 
% \end{array},
% \end{equation}

% \section{force coefficient matrices}
% $\Lambda_K$ allows convenient gain tuning of the individual components.
